# Supplementary material for: A Novel Classification Approach for Credit Scoring based on Gaussian Mixture Models
Source: arXiv:2010.13388 source file (2020-10-26)
Supplement: Supplementary file 1 [file appendix.tex]

\section{Appendix}
