# Supplementary material for: A Novel Classification Approach for Credit Scoring based on Gaussian Mixture Models
Source: arXiv:2010.13388 source file (2020-10-26)
Supplement: Supplementary file 2 [file appendixweb.tex]

\section{Web Appendix}
\begin{table}
  \label{datahead}
  \centering
  \caption{Data of German}
\begin{tabular}{lcccccc}
    \toprule
    \textbf{existingchecking} & \textbf{duration} & \textbf{credithistory} & \textbf{purpose} & \textbf{creditamount} & \textbf{savings} & \textbf{employmentsince} \\
    \midrule
    A11   & 6     & A34   & A43   & 1169  & A65   & A75 \\
    A12   & 48    & A32   & A43   & 5951  & A61   & A73 \\
    A14   & 12    & A34   & A46   & 2096  & A61   & A74 \\
    A11   & 42    & A32   & A42   & 7882  & A61   & A74 \\
    A11   & 24    & A33   & A40   & 4870  & A61   & A73 \\
    \toprule
    \textbf{installmentrate} & \textbf{statussex} & \textbf{otherdebtors} & \textbf{residencesince} & \textbf{property} & \textbf{age}   & \textbf{otherinstallmentplans} \\
    \midrule
    4     & A93   & A101  & 4     & A121  & 67    & A143 \\
    2     & A92   & A101  & 2     & A121  & 22    & A143 \\
    2     & A93   & A101  & 3     & A121  & 49    & A143 \\
    2     & A93   & A103  & 4     & A122  & 45    & A143 \\
    3     & A93   & A101  & 4     & A124  & 53    & A143 \\
    \toprule
    \textbf{housing} & \textbf{existingcredits} & \textbf{job}   & \textbf{peopleliable} & \textbf{telephone} & \textbf{foreignworker} & \textbf{classification} \\
    \midrule
    A152  & 2     & A173  & 1     & A192  & A201  & 1 \\
    A152  & 1     & A173  & 1     & A191  & A201  & 2 \\
    A152  & 1     & A172  & 2     & A191  & A201  & 1 \\
    A153  & 1     & A173  & 2     & A191  & A201  & 1 \\
    A153  & 2     & A173  & 2     & A191  & A201  & 2 \\
    \bottomrule
    \end{tabular}%
\end{table}%
